# Supplementary material for: Analyzing and Debugging Normative Requirements via Satisfiability Checking
Source: arXiv:2401.05673 source file (2024-01-11)
Supplement: Supplementary file 1 [file appendix-evaluation-protocol.tex]

\subsection{Evaluation Protocol}
% header
The objective of the evaluation protocol is twofold. First, it aims to assess the relevance of identified \CRRI issues, including vacuous-, situational-conflicts, redundancy, insufficiency, and restrictiveness, within each case study. Second, it aims to evaluate the usability of the diagnosis for resolving the identified \CRRI issues. For each type of issue identified, the following questions should be posed to the stakeholders:

%\boldparagraph{Case study processing}
%\begin{itemize}
%    \item Are all the events, 
%\end{itemize}

\boldparagraph{Relevance of \CRRI issues and diagnostics}
\begin{enumerate}
\item Do you understand the \CRRI issues? Please respond with 'yes', 'no', or 'not sure'.
\item If 'yes', is the issue relevant or spurious? If you consider it spurious, please provide a justification.
\item If the \CRRI issue is not considered spurious, was the diagnostic information useful for understanding the problem? Please respond with 'yes' or 'no'.
\item If the \CRRI issue is not considered spurious, can the diagnosis be used to resolve it? If so, please provide details on how it can be resolved.
\item Which aspect of the diagnostic was unhelpful? Was it the highlighted rules, the trace, or the measure values?
\item If the inconsistency cannot be resolved, is it due to the diagnosis lacking sufficient assistance? If so, please specify what is lacking. Alternatively, is it determined to be impossible to resolve the inconsistency? If so, please explain the reason.
\item Is there an \CRRI issue that you believe we did not capture?
\end{enumerate}

\boldparagraph{Global feedback}
\begin{itemize}
    \item Do you have any feedback regarding the strengths of the proposed approach?
    \item Do you have any feedback regarding the weaknesses of the proposed approach?
    \item Do you have any feedback regarding the strengths of the produced diagnosis?
    \item Do you have any feedback regarding the weaknesses of the produced diagnosis?
    \item Do you have any additional needs you encountered that could benefit from formal automated tool assistance?
\end{itemize}
